# Supplementary material for: Rooting Out Letters: Octagonal Symbol Alphabets and Algebraic Number Theory
Source: arXiv:1910.14224 ancillary file (2019-10-31)
Supplement: Supplementary file 1 [file PrimeFactorLetters.pdf]

|              | 2 | 3 | 5 | 7 | 11 | 13 | 17 | 23 | 29 | 31 | 37 | 41 | 43 | 47 | 53* | 61 | 67 | 71 | 89 | 113 | 173 | 269 | 271 | 283 | 337 | 431 | 769 | 1217 | 1549 | 4517* | 5347* |
|--------------|---|---|---|---|----|----|----|----|----|----|----|----|----|----|-----|----|----|----|----|-----|-----|-----|-----|-----|-----|-----|-----|------|------|-------|-------|
| (1, 2, 3, 4) |   |   |   |   |    |    |    |    |    |    |    |    |    |    |     |    |    |    |    |     |     |     |     |     |     |     |     |      |      |       |       |
| (1, 2, 3, 5) | 1 |   |   |   | 1  |    |    |    |    |    |    |    |    |    |     |    |    |    |    |     |     |     |     |     |     |     |     |      |      |       |       |
| (1, 2, 3, 6) |   | 1 |   |   |    |    |    |    |    |    |    |    |    |    |     |    |    |    |    |     |     |     |     |     |     |     |     |      |      |       |       |
| (1, 2, 3, 7) | 3 |   |   |   |    |    |    |    |    |    |    |    |    |    |     |    |    |    |    |     |     |     |     |     |     |     |     |      |      |       |       |
| (1, 2, 3, 8) |   |   |   |   |    |    |    |    |    |    |    |    |    |    |     |    |    |    |    |     |     |     |     |     |     |     |     |      |      |       |       |
| (1, 2, 4, 5) |   | 1 |   |   |    |    |    |    |    |    |    |    |    |    |     |    |    |    |    |     |     |     |     |     |     |     |     |      |      |       |       |
| (1, 2, 4, 6) |   |   |   |   |    |    |    |    |    |    |    |    |    |    |     |    |    |    |    |     |     |     |     |     |     |     |     |      |      |       |       |
| (1, 2, 4, 7) |   |   |   | 1 |    |    |    |    |    |    |    |    |    |    |     |    |    |    |    |     |     |     |     |     |     |     |     |      |      |       |       |
| (1, 2, 4, 8) |   |   |   |   |    |    |    |    |    |    |    |    |    |    |     |    |    |    |    |     |     |     |     |     |     |     |     |      |      |       |       |
| (1, 2, 5, 6) |   | 1 |   |   |    |    |    |    |    |    |    |    |    |    |     |    |    |    |    |     |     |     |     |     |     |     |     |      |      |       |       |
| (1, 2, 5, 7) | 1 |   |   |   |    |    |    |    |    |    | 1  |    |    |    |     |    |    |    |    |     |     |     |     |     |     |     |     |      |      |       |       |
| (1, 2, 5, 8) |   |   |   |   | 1  |    |    |    |    |    |    |    |    |    |     |    |    |    |    |     |     |     |     |     |     |     |     |      |      |       |       |
| (1, 2, 6, 7) |   |   |   |   |    | 1  |    |    |    |    |    |    |    |    |     |    |    |    |    |     |     |     |     |     |     |     |     |      |      |       |       |
| (1, 2, 6, 8) | 1 |   |   |   |    |    |    |    |    |    |    |    |    |    |     |    |    |    |    |     |     |     |     |     |     |     |     |      |      |       |       |
| (1, 2, 7, 8) |   |   |   |   |    |    |    |    |    |    |    |    |    |    |     |    |    |    |    |     |     |     |     |     |     |     |     |      |      |       |       |
| (1, 3, 4, 5) |   |   |   | 1 |    |    |    |    |    |    |    |    |    |    |     |    |    |    |    |     |     |     |     |     |     |     |     |      |      |       |       |
| (1, 3, 4, 6) | 1 | 1 |   |   |    |    |    |    |    |    |    |    |    |    |     |    |    |    |    |     |     |     |     |     |     |     |     |      |      |       |       |
| (1, 3, 4, 7) | 1 |   |   |   |    |    |    |    |    |    | 1  |    |    |    |     |    |    |    |    |     |     |     |     |     |     |     |     |      |      |       |       |
| (1, 3, 4, 8) |   |   |   |   | 1  |    |    |    |    |    |    |    |    |    |     |    |    |    |    |     |     |     |     |     |     |     |     |      |      |       |       |
| (1, 3, 5, 6) |   | 2 |   | 1 |    |    |    |    |    |    |    |    |    |    |     |    |    |    |    |     |     |     |     |     |     |     |     |      |      |       |       |
| (1, 3, 5, 8) | 1 |   | 2 |   |    |    |    |    |    |    |    |    |    |    |     |    |    |    |    |     |     |     |     |     |     |     |     |      |      |       |       |
| (1, 3, 6, 7) | 1 | 1 |   |   |    |    |    |    | 1  |    |    |    |    |    |     |    |    |    |    |     |     |     |     |     |     |     |     |      |      |       |       |
| (1, 3, 6, 8) |   | 3 |   |   |    |    |    |    |    |    |    |    |    |    |     |    |    |    |    |     |     |     |     |     |     |     |     |      |      |       |       |
| (1, 3, 7, 8) | 1 |   |   |   | 1  |    |    |    |    |    |    |    |    |    |     |    |    |    |    |     |     |     |     |     |     |     |     |      |      |       |       |
| (1, 4, 5, 6) |   |   |   |   |    | 1  |    |    |    |    |    |    |    |    |     |    |    |    |    |     |     |     |     |     |     |     |     |      |      |       |       |
| (1, 4, 5, 7) |   |   |   |   |    |    |    |    |    |    |    |    |    |    |     |    |    |    |    |     | 1   |     |     |     |     |     |     |      |      |       |       |
| (1, 4, 5, 8) | 1 |   |   |   |    | 1  |    |    |    |    |    |    |    |    |     |    |    |    |    |     |     |     |     |     |     |     |     |      |      |       |       |
| (1, 4, 6, 7) | 5 |   |   |   |    |    |    |    |    |    |    |    |    |    |     |    |    |    |    |     |     |     |     |     |     |     |     |      |      |       |       |
| (1, 4, 6, 8) |   | 1 |   |   |    |    |    |    |    |    |    |    |    |    |     |    |    |    |    |     |     |     |     |     |     |     |     |      |      |       |       |
| (1, 4, 7, 8) | 1 |   |   |   |    |    |    |    |    |    |    |    |    |    |     |    |    |    |    |     |     |     |     |     |     |     |     |      |      |       |       |
| (1, 5, 6, 7) |   |   |   |   |    |    | 1  |    |    |    |    |    |    |    |     |    |    |    |    |     |     |     |     |     |     |     |     |      |      |       |       |
| (1, 5, 6, 8) |   | 1 |   |   |    |    |    |    |    |    |    |    |    |    |     |    |    |    |    |     |     |     |     |     |     |     |     |      |      |       |       |
| (1, 5, 7, 8) |   |   |   | 1 |    |    |    |    |    |    |    |    |    |    |     |    |    |    |    |     |     |     |     |     |     |     |     |      |      |       |       |
| (1, 6, 7, 8) |   |   |   |   |    |    |    |    |    |    |    |    |    |    |     |    |    |    |    |     |     |     |     |     |     |     |     |      |      |       |       |
| (2, 3, 4, 5) |   |   |   |   |    |    |    |    |    |    |    |    |    |    |     |    |    |    |    |     |     |     |     |     |     |     |     |      |      |       |       |
| (2, 3, 4, 6) |   |   |   |   |    |    |    |    |    |    |    |    |    |    |     |    |    |    |    |     |     |     |     |     |     |     |     |      |      |       |       |
| (2, 3, 4, 7) |   |   |   |   |    | 1  |    |    |    |    |    |    |    |    |     |    |    |    |    |     |     |     |     |     |     |     |     |      |      |       |       |
| (2, 3, 4, 8) | 1 |   |   |   |    |    |    |    |    |    |    |    |    |    |     |    |    |    |    |     |     |     |     |     |     |     |     |      |      |       |       |
| (2, 3, 5, 6) |   |   |   |   | 1  |    |    |    |    |    |    |    |    |    |     |    |    |    |    |     |     |     |     |     |     |     |     |      |      |       |       |
| (2, 3, 5, 7) | 1 | 1 |   |   |    |    |    |    | 1  |    |    |    |    |    |     |    |    |    |    |     |     |     |     |     |     |     |     |      |      |       |       |
| (2, 3, 5, 8) |   | 3 |   |   |    |    |    |    |    |    |    |    |    |    |     |    |    |    |    |     |     |     |     |     |     |     |     |      |      |       |       |
| (2, 3, 6, 7) |   |   |   |   |    |    |    |    |    |    | 1  |    |    |    |     |    |    |    |    |     |     |     |     |     |     |     |     |      |      |       |       |
| (2, 3, 6, 8) |   |   | 1 |   |    |    |    |    |    |    |    |    |    |    |     |    |    |    |    |     |     |     |     |     |     |     |     |      |      |       |       |
| (2, 3, 7, 8) |   | 1 |   |   |    |    |    |    |    |    |    |    |    |    |     |    |    |    |    |     |     |     |     |     |     |     |     |      |      |       |       |
| (2, 4, 5, 6) | 1 |   |   |   |    |    |    |    |    |    |    |    |    |    |     |    |    |    |    |     |     |     |     |     |     |     |     |      |      |       |       |
| (2, 4, 5, 7) | 5 |   |   |   |    |    |    |    |    |    |    |    |    |    |     |    |    |    |    |     |     |     |     |     |     |     |     |      |      |       |       |
| (2, 4, 5, 8) |   |   | 1 |   |    |    |    |    |    |    |    |    |    |    |     |    |    |    |    |     |     |     |     |     |     |     |     |      |      |       |       |
| (2, 4, 6, 7) | 1 | 1 |   |   |    |    |    |    |    |    |    |    |    |    |     |    |    |    |    |     |     |     |     |     |     |     |     |      |      |       |       |
| (2, 4, 7, 8) |   |   |   |   |    |    |    |    |    |    |    |    |    |    |     |    |    |    |    |     |     |     |     |     |     |     |     |      |      |       |       |
| (2, 5, 6, 7) | 2 |   |   |   |    |    |    |    |    |    |    |    |    |    |     |    |    |    |    |     |     |     |     |     |     |     |     |      |      |       |       |
| (2, 5, 6, 8) |   |   |   |   |    |    |    |    |    |    |    |    |    |    |     |    |    |    |    |     |     |     |     |     |     |     |     |      |      |       |       |
| (2, 5, 7, 8) | 1 | 1 |   |   |    |    |    |    |    |    |    |    |    |    |     |    |    |    |    |     |     |     |     |     |     |     |     |      |      |       |       |
| (2, 6, 7, 8) |   |   |   |   |    |    |    |    |    |    |    |    |    |    |     |    |    |    |    |     |     |     |     |     |     |     |     |      |      |       |       |
| (3, 4, 5, 6) |   |   |   |   |    |    |    |    |    |    |    |    |    |    |     |    |    |    |    |     |     |     |     |     |     |     |     |      |      |       |       |
| (3, 4, 5, 7) |   |   |   |   |    |    | 1  |    |    |    |    |    |    |    |     |    |    |    |    |     |     |     |     |     |     |     |     |      |      |       |       |
| (3, 4, 5, 8) |   | 1 |   |   |    |    |    |    |    |    |    |    |    |    |     |    |    |    |    |     |     |     |     |     |     |     |     |      |      |       |       |
| (3, 4, 6, 7) | 2 |   |   |   |    |    |    |    |    |    |    |    |    |    |     |    |    |    |    |     |     |     |     |     |     |     |     |      |      |       |       |



[illegible]
